# Supplementary material for: Machine Learning Assisted Cognitive Construction of a Shallow Depth Dynamic Ansatz for Noisy Quantum Hardware
Source: arXiv:2310.08468 ancillary file (2023-10-12)
Supplement: Supplementary file 1 [file supplementary_information.pdf]

# Supplementary Material for “Machine Learning Assisted Cognitive Construction of a Shallow Depth Dynamic Ansatz for Noisy Quantum Hardware”

Sonaldeep Halder, Anish Dey, Chinmay Shrikhande, and Rahul Maitra

## S1. Details of Restricted Boltzmann Machines

### A. Training and generating procedure

1. The configurations and their corresponding probabilities from the computational state basis are extracted after converging the energy variationally using single and double excitations pruned at the MP2 level (dUCCSD ansatz as described in section **II a** of the main article). The configurations with probabilities greater than $10^{-5}$ are considered for our dataset. While using statevector, exact probabilities are taken, whereas when using *shot-based* simulators (where expectation values are calculated through repeated measurements), the probabilities are obtained through measurements.
2. These configurations are used to generate a training set of 500000 points based on their corresponding probabilities. Sklearn's BernoulliRBM is used for training on the dataset. The hyperparameters of our model are given below:
   Number of hidden nodes = 30
   Learning rate = 0.01
   Number of iterations = 30
   Batch Size = 10
3. The trained parameters of the model are obtained after training. The activation probabilities of the hidden layer are used further to get the activation probabilities of the visible layer by utilizing the model's parameters. Parameters are estimated using Persistent Contrastive Divergence.
4. The "Tower Sampling Algorithm" is deployed to ensure the total spin and number of particles are conserved.
5. The tower sampled data is Gibbs Sampled for two consecutive steps to get a transformed data set. Decreasing the number of Gibbs sampling introduces more noise into the generated data, whereas increasing the number of Gibbs sampling steps makes the generated data more like the training data.
6. This study focuses on triples therefore, only the triples are extracted from the generated data. This method can be extended to other higher-excited configurations as well.
7. MP2 values are used as a measure to take into account the most dominant triples, as described in section **II C** of our main article.
8. The ansatz is updated accordingly, and the newly generated dominant triples are added to the existing training dataset. The steps from 2-9 are repeated until our model ceases to generate useful triples for 6 iterations consecutively.

## B. A Brief Description of Tower Sampling

Suppose we have the activation probabilities of the visible layer ( qubit size/dimension of visible layer = 10, number of electrons = 4)

| 0 | 1 | 2 | 3 | 4 | 5 | 6 | 7 | 8 | 9 |
|---|---|---|---|---|---|---|---|---|---|
| 0.01 | 0.02 | 0.05 | 0.1 | 0.5 | 0.37 | 0.12 | 0.45 | 0.78 | 0.04 |

The first 5 units of the visible layer correspond to α set of spin orbitals and the later corresponds to β set of spin orbitals. To ensure that only 2 electrons (number conservation) are present in each of these halves (spin conservation), this sampling method is used. We use the algorithm on each of these halves separately.

1. A tower of height $\sum_{i=0}^{n} P_{\mathrm{i}}$ is constructed with the height of each block to be the activation probability of each unit of the visible layer (here n=4) -

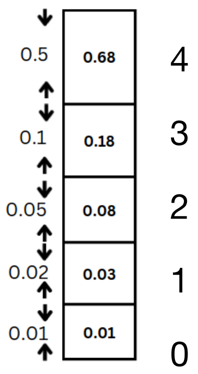


2. A random number between 0 and $\sum_{i=0}^{4} P_{\mathrm{i}}$ (height of the tower) is generated. Suppose the random number comes out to be 0.04. This lies in the 3rd block of the tower. The electron is filled in the 3rd block (label of index 2) -

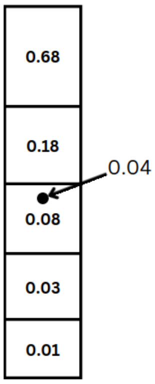

3. A new tower is constructed with the probabilities of the remaining 4 units. Steps 1 to 3 are repeated until we have exhausted all the electrons (here, in this case, the number =2 ).

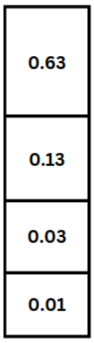


The same is done for the set of β orbitals.

## S2. A brief discussion on *scatterer* operators

A more formal description regarding the *scatterers* can be obtained from the work of Halder et al. [1], where they highlight the generation of higher-order excitations as an outcome of operator non-commutativity and disentangled (factorized) structure of the unitary through a set of exponentiated nested commutator terms.

$$e^{\hat{\sigma}}e^{\hat{\kappa}} = e^{(\hat{\sigma}+\hat{\kappa})+[\hat{\sigma},\hat{\kappa}]+\dots} \tag{1}$$

If $\hat{\kappa}^D$ represents a rank two excitation operator, the commutator in Eq. (1) results in the generation of a rank three excitation operator ($\hat{\kappa}^T$):

$$[\hat{\sigma}, \hat{\kappa}^D] \longrightarrow \hat{\kappa}^T \tag{2}$$

Multiple exponentiated *scatterers* can act consecutively over the same low-rank excitation operator to generate excited configurations that may differ by more than rank one. This occurs due to the nested commutator that arises in such cases.

$$\begin{aligned} e^{\hat{\sigma}_2}e^{\hat{\sigma}_1}e^{\hat{\kappa}} &= e^{\hat{\sigma}_2}e^{(\hat{\sigma}_1+\hat{\kappa})+[\hat{\sigma}_1,\hat{\kappa}]+\dots} \\ &= e^{\hat{\sigma}_2+\hat{\sigma}_1+\hat{\kappa}+[\hat{\sigma}_2,\hat{\kappa}]+[\hat{\sigma}_1,\hat{\kappa}]+[\hat{\sigma}_2,[\hat{\sigma}_1,\hat{\kappa}]]+\dots} \end{aligned} \tag{3}$$

If $\hat{\kappa}^D$ represents a rank two excitation operator, the commutators in Eq. (3) result in different rank three excitation operators and even other higher rank excitation operators such as quadruples ($\hat{\kappa}^Q$) depending on the excitation structure of the two *scatterers* ($\sigma_1$ and $\sigma_2$).

$$\begin{aligned} [\hat{\sigma}_1, \hat{\kappa}^D] &\longrightarrow \hat{\kappa}_1^T \\ [\hat{\sigma}_2, \hat{\kappa}^D] &\longrightarrow \hat{\kappa}_2^T \\ [\hat{\sigma}_2, [\hat{\sigma}_1, \hat{\kappa}^D]] &\longrightarrow \hat{\kappa}^Q \end{aligned} \tag{4}$$

Eq. (4) is also provided in the main article.

## References

[1] D. Halder, V. Prasannaa, and R. Maitra, "Dual exponential coupled cluster theory: unitary adaptation, implementation in the variational quantum eigensolver framework and pilot applications", The Journal of Chemical Physics **157** (2022).
